# Supplementary material for: Competition of Density Waves and Superconductivity in Twisted Tungsten Diselenide
Source: arXiv:2204.00648 source file (2023-03-14)
Supplement: Supplementary file 1 [file supp.pdf]

## Supplemental Material

### Competition of Density Waves and Superconductivity in Twisted Tungsten Diselenide

Lennart Klebl,<sup>1</sup> Ammon Fischer,<sup>1</sup> Laura Classen,<sup>2</sup> Michael M. Scherer,<sup>3</sup> and Dante M. Kennes<sup>1,4</sup>

<sup>1</sup>*Institut für Theorie der Statistischen Physik, RWTH Aachen University and JARA-Fundamentals of Future Information Technology, D-52056 Aachen, Germany*

<sup>2</sup>*Max Planck Institute for Solid State Research, D-70569 Stuttgart, Germany*

<sup>3</sup>*Institut für Theoretische Physik III, Ruhr-Universität Bochum, D-44801 Bochum, Germany*

<sup>4</sup>*Max Planck Institute for the Structure and Dynamics of Matter, Center for Free Electron Laser Science, D-22761 Hamburg, Germany*

(Dated: April 1, 2022)

#### SI. FUNCTIONAL RENORMALIZATION GROUP IN NON- $SU(2)$ SYSTEMS

The supplementary material aims to provide the most relevant concepts and equations of the functional renormalization group study applied in the main text. First, we show the flow equations of the fermionic four-point vertex  $\Gamma^{(4)}$  in the absence of  $SU(2)$  symmetry and afterwards describe in detail how to post-process the vertex to obtain information about the spin/charge and superconducting instabilities in the system. In parts, we follow the description published in the Method Section of Ref. S1.

We approximate the formally exact functional renormalization group by discarding self-energies, frequency dependencies of the four-point vertex, and vertices with more than four legs. The method smoothly interpolates from the non-interacting theory at infinite scale  $\Lambda$  to the fully interacting theory at  $\Lambda = 0$ . In our implementation, we employ a sharp cutoff on the Green's function such

that

$$G_{\sigma\sigma'}^{\Lambda}(ik_0, \mathbf{k}) = \Theta(|ik_0| - \Lambda) G_{\sigma\sigma'}^0(ik_0, \mathbf{k}). \quad (\text{S1})$$

Here,  $\hat{G}^0(ik_0, \mathbf{k}) = (ik_0 - \hat{H}^0(\mathbf{k}))^{-1}$  is the non-interacting Green's function as a matrix in spin space. With this scale-dependent propagator, we derive an ordinary differential equation for the four-point vertex function  $\Gamma^{(4),\Lambda}$  [S2–S4] that is visualized diagrammatically in Fig. S1. The resulting equations read

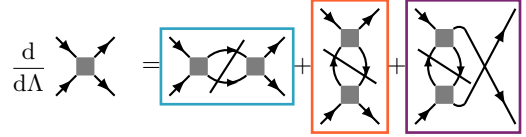

FIG. S1. Diagrammatic form of the non- $SU(2)$  symmetric flow equations for the four-point vertex  $\Gamma^{(4)}$ . Slashed propagator lines refer to the single-scale propagator.

$$\frac{d}{d\Lambda} \Gamma^{(4),\Lambda} = \frac{d}{d\Lambda} (P^{\Lambda} + D^{\Lambda} + C^{\Lambda}), \quad (\text{S2})$$

$$\frac{d}{d\Lambda} P_{\sigma_1\sigma_2\sigma_3\sigma_4}^{\Lambda}(\mathbf{q}_P, \mathbf{k}_P, \mathbf{k}'_P) = \frac{1}{2} \sum_{\mathbf{k}\sigma_{3'}\sigma_{4'}\sigma_{1'}\sigma_{2'}} \Gamma_{\sigma_1\sigma_2\sigma_{3'}\sigma_{4'}}^{P,\Lambda}(\mathbf{q}_P, \mathbf{k}_P, \mathbf{k}) \frac{d}{d\Lambda} L_{\sigma_{3'}\sigma_{4'}\sigma_{1'}\sigma_{2'}}^{P,\Lambda}(\mathbf{q}_P, \mathbf{k}) \Gamma_{\sigma_{1'}\sigma_{2'}\sigma_3\sigma_4}^{P,\Lambda}(\mathbf{q}_P, \mathbf{k}, \mathbf{k}'_P), \quad (\text{S3})$$

$$\frac{d}{d\Lambda} D_{\sigma_1\sigma_2\sigma_3\sigma_4}^{\Lambda}(\mathbf{q}_D, \mathbf{k}_D, \mathbf{k}'_D) = - \sum_{\mathbf{k}\sigma_{3'}\sigma_{4'}\sigma_{1'}\sigma_{2'}} \Gamma_{\sigma_1\sigma_2\sigma_{3'}\sigma_{4'}}^{D,\Lambda}(\mathbf{q}_D, \mathbf{k}_D, \mathbf{k}) \frac{d}{d\Lambda} L_{\sigma_{3'}\sigma_{4'}\sigma_{1'}\sigma_{2'}}^{D,\Lambda}(\mathbf{q}_D, \mathbf{k}) \Gamma_{\sigma_{1'}\sigma_{2'}\sigma_3\sigma_4}^{D,\Lambda}(\mathbf{q}_D, \mathbf{k}, \mathbf{k}'_D), \quad (\text{S4})$$

$$\frac{d}{d\Lambda} C_{\sigma_1\sigma_2\sigma_3\sigma_4}^{\Lambda}(\mathbf{k}_1, \mathbf{k}_2, \mathbf{k}_3) = - \frac{d}{d\Lambda} D_{\sigma_1\sigma_2\sigma_4\sigma_3}^{\Lambda}(\mathbf{k}_1, \mathbf{k}_2, \mathbf{k}_1 + \mathbf{k}_2 - \mathbf{k}_3). \quad (\text{S5})$$

Here, the channel-projections to the particle-particle ( $P$ ), and direct particle-hole ( $D$ ) channels read

$$\Gamma_{\sigma_1\sigma_2\sigma_3\sigma_4}^{P,\Lambda}(\mathbf{q}_P, \mathbf{k}_P, \mathbf{k}'_P) = \Gamma_{\sigma_1\sigma_2\sigma_3\sigma_4}^{(4),\Lambda}(\mathbf{k}_1, \mathbf{k}_2, \mathbf{k}_3), \quad (\text{S6})$$

$$\Gamma_{\sigma_1\sigma_2\sigma_3\sigma_4}^{D,\Lambda}(\mathbf{q}_D, \mathbf{k}_D, \mathbf{k}'_D) = \Gamma_{\sigma_3\sigma_1\sigma_2\sigma_4}^{(4),\Lambda}(\mathbf{k}_1, \mathbf{k}_2, \mathbf{k}_3). \quad (\text{S7})$$

The bosonic momentum  $\mathbf{q}_X$  and the two fermionic mo-

menta  $\mathbf{k}_X, \mathbf{k}'_X$  are transformed as

$$\mathbf{q}_P = \mathbf{k}_1 + \mathbf{k}_2, \quad \mathbf{k}_P = \mathbf{k}_1, \quad \mathbf{k}'_P = \mathbf{k}_3, \quad (\text{S8})$$

$$\mathbf{q}_D = \mathbf{k}_1 - \mathbf{k}_3, \quad \mathbf{k}_D = \mathbf{k}_1, \quad \mathbf{k}'_D = \mathbf{k}_1 + \mathbf{k}_2 - \mathbf{k}_3. \quad (\text{S9})$$

Here, the momenta  $\mathbf{k}_{1,2,3}$  refer to the indices of the vertex function in standard ordering with 1, 2 incoming and

3, 4 outgoing legs. The scale-derivatives in the corresponding channels in Eqs. (S3) and (S4) are written with the respective bosonic and fermionic momentum indices,

$$\frac{d}{d\Lambda} L_{\sigma_1 \sigma_2 \sigma_3 \sigma_4}^{P, \Lambda}(\mathbf{q}^P, \mathbf{k}_1) = \frac{1}{2\pi} \sum_{b_1 b_2} u_{\sigma_1 b_1}(\mathbf{k}_1) u_{\sigma_3 b_1}^*(\mathbf{k}_1) u_{\sigma_2 b_2}(\mathbf{k}_2^P) u_{\sigma_4 b_2}^*(\mathbf{k}_2^P) \times \quad (S10)$$

$$\left[ \frac{1}{(-i\Lambda - \epsilon_{b_1}(\mathbf{k}_1))(i\Lambda - \epsilon_{b_2}(\mathbf{k}_2^P))} + \frac{1}{(i\Lambda - \epsilon_{b_1}(\mathbf{k}_1))(-i\Lambda - \epsilon_{b_2}(\mathbf{k}_2^P))} \right],$$

$$\frac{d}{d\Lambda} L_{\sigma_4 \sigma_1 \sigma_2 \sigma_3}^{D, \Lambda}(\mathbf{q}^D, \mathbf{k}_1) = \frac{1}{2\pi} \sum_{b_1 b_2} u_{\sigma_1 b_1}(\mathbf{k}_1) u_{\sigma_3 b_1}^*(\mathbf{k}_1) u_{\sigma_2 b_2}(\mathbf{k}_2^D) u_{\sigma_4 b_2}^*(\mathbf{k}_2^D) \times \quad (S11)$$

$$\left[ \frac{1}{(i\Lambda - \epsilon_{b_1}(\mathbf{k}_1))(i\Lambda - \epsilon_{b_2}(\mathbf{k}_2^D))} + \frac{1}{(-i\Lambda - \epsilon_{b_1}(\mathbf{k}_1))(-i\Lambda - \epsilon_{b_2}(\mathbf{k}_2^D))} \right],$$

where we defined the channel-dependent momentum differences  $\mathbf{k}_2^P = \mathbf{q}^P - \mathbf{k}_1$  and  $\mathbf{k}_2^D = \mathbf{q}^D + \mathbf{k}_1$ .  $u_{\sigma b}(\mathbf{k})$  denote Bloch functions of the single-particle tight-binding Hamiltonian with dispersion  $\epsilon_b(\mathbf{k})$ .

Technically, we discretize momentum space for the vertex functions with a  $24 \times 24$  meshing of the reciprocal primitive zone. The Green's functions (and loops) are calculated on a much finer mesh with 649 points for each of the  $24 \times 24$  points. In order to preserve symmetries, the fine points are chosen in the Wigner-Seitz cells defined by the coarse mesh. An instructive description of this meshing procedure is found in Ref. S5. The central differential equation (in  $\Lambda$ ) is integrated with an enhanced adaptive Euler scheme that first constrains the step size to be 10% of the current  $\Lambda$  at maximum and further scales the step size inversely to the maximum value of  $\Gamma^{(4), \Lambda}$ . We consider the flow as diverged when the maximum absolute value of a vertex component is larger than  $30t$ . From the value at which this divergence occurs, we obtain the critical scale  $\Lambda_c$  and by inspection of the channel that contributes most strongly to the divergence of  $\Gamma^{(4), \Lambda}$  whether a particle-particle ( $P$ ) or a particle-hole ( $D, C$ ) instability is present.

### SII. FUNCTIONAL RENORMALIZATION GROUP FLOWS

For selected points along the  $\nu = 0$  vertical line in the phase diagram (Fig. 1 of the main text), we plot the channel contribution maxima and the vertex maximum as a function of  $\Lambda$  to visualize the pronounced tendency towards order in Fig. S2. We define the channel contribution maximum  $X_{\max}^\Lambda$  of channel  $X \in P, C, D$  as

$$X_{\max}^\Lambda = \max_{\mathbf{k}_1 \mathbf{k}_2 \mathbf{k}_3, s_1 \dots s_4} \left| d\Lambda \frac{dX^\Lambda}{d\Lambda} \right|, \quad (S12)$$

whereas Eq. (S5) refers to fermionic indices in standard ordering. The loop contributions in Eqs. (S3) and (S4) can be written as

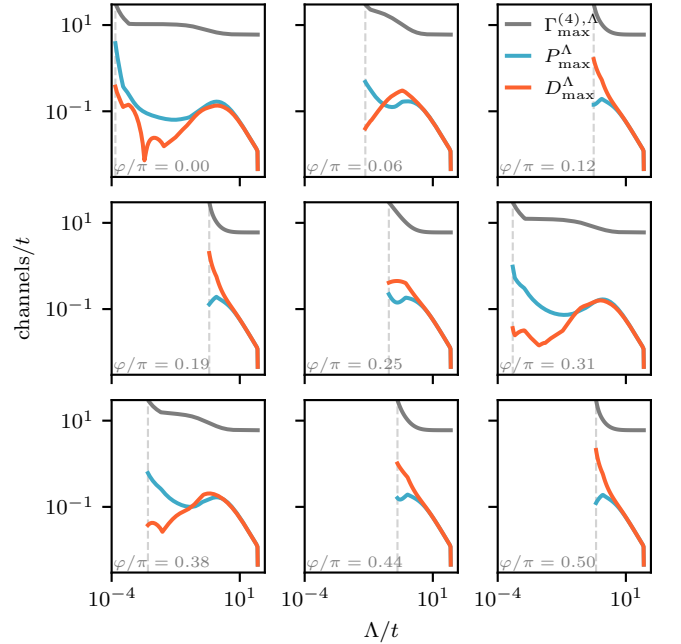

FIG. S2. Channel maxima as a function of the RG scale  $\Lambda$  for  $\nu = 0$  and varied  $\varphi$  (bottom left of each panel). Blue curves denote the  $P$ -channel maximum, orange curves the  $D$ -channel maximum and gray curves the vertex maximum. The dashed gray line shows the value of  $\Lambda_c$ .

where the expression  $dX^\Lambda/d\Lambda$  is numerically obtained from Eqs. (S3) to (S5). Note that  $C_{\max}^\Lambda \equiv D_{\max}^\Lambda$  as in the non- $SU(2)$  case, these two channels are connected via reordering of the third and fourth vertex index. As the onset of strong correlations is signaled by a divergence of  $V^\Lambda$  at  $\Lambda_c$ , we can inspect the type of order by comparing  $D_{\max}^\Lambda$  with  $P_{\max}^\Lambda$  at  $\Lambda \lesssim \Lambda_c$  – the behavior close to the divergence indicates which order (i.e. particle-hole ( $D$ ) or particle-particle ( $P$ )) eventually dominates.

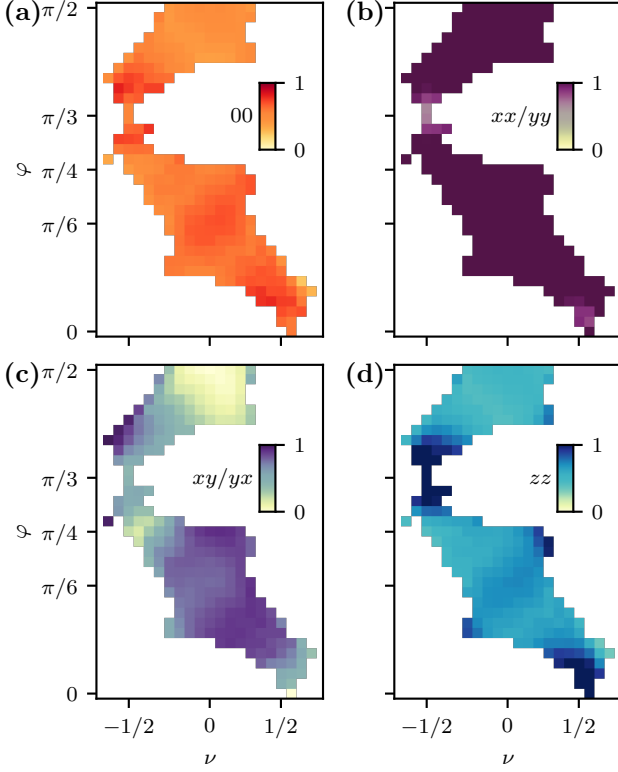

FIG. S3. **Spin and Density weights of the particle-hole instabilities.** For each  $\nu$  and  $\varphi$  where our FRG analysis predicts DW order, we calculated the weight function  $w(i, j)$  in spin/density space and normalize by its maximum value. We color-code this information for the four non-trivial spin/density correlations. This analysis visualizes that at no point, the density-density correlation (a) is dominant, and that for almost all other points, the spin- $xx/yy$  correlation (b) dominates over the spin- $zz$  correlation (d) and the spin- $xy/yx$  correlation (c).

### SIII. ANALYSIS OF SPIN/DENSITY-WAVE PHASES

In the case of particle-hole instabilities, the resulting ordered phase generally mixes spin with density order due to the non- $SU(2)$  nature of the system. Further analysis of the instability is provided by the calculation of four-point susceptibilities, detailed in the following.

#### SIII. A. Four-point susceptibilities

The interacting four-point particle-hole susceptibility  $\chi_{\sigma_1\sigma_2\sigma_3\sigma_4}^D(\mathbf{q}_D)$  at scale  $\Lambda_c$  is obtained from a two-loop diagram with all fermionic momenta being contracted:

$$\chi_{\sigma_1\sigma_2\sigma_3\sigma_4}^D(\mathbf{q}_D) = \sum_{\mathbf{k}_D \mathbf{k}'_D \sigma_1' \sigma_2' \sigma_3' \sigma_4'} L_{\sigma_1\sigma_2\sigma_1'\sigma_2'}^{f,D,\Lambda_c}(\mathbf{q}_D, \mathbf{k}_D) \Gamma_{\sigma_1'\sigma_2'\sigma_3'\sigma_4'}^{D,\Lambda_c}(\mathbf{q}_D, \mathbf{k}_D, \mathbf{k}'_D) L_{\sigma_3'\sigma_4'\sigma_3\sigma_4}^{f,D,\Lambda_c}(\mathbf{q}_D, \mathbf{k}'_D). \quad (\text{S13})$$

The loop function at scale  $\Lambda$  reads

$$L_{\sigma_4\sigma_1\sigma_2\sigma_3}^{f,D,\Lambda}(\mathbf{q}^D, \mathbf{k}_1) = \sum_{b_1 b_2} \frac{u_{\sigma_1 b_1}(\mathbf{k}_1) u_{\sigma_3 b_1}^*(\mathbf{k}_1) u_{\sigma_2 b_2}(\mathbf{k}_2^D) u_{\sigma_4 b_2}^*(\mathbf{k}_2^D) [f(\epsilon_{b_1}(\mathbf{k}_1)/\Lambda) - f(\epsilon_{b_2}(\mathbf{k}_2^D)/\Lambda)]}{\epsilon_{b_1}(\mathbf{k}_1) - \epsilon_{b_2}(\mathbf{k}_2^D)}, \quad (\text{S14})$$

which is nothing else but the non-interacting four-point particle-hole susceptibility  $\chi_{s_1 \dots s_4}^{0,\Lambda}(\mathbf{q}^D, \mathbf{k}_1) = \sum_{i(k_1)_0} G_{s_1 s_3}^0(k_1) G_{s_2 s_4}^0(k_1 + \mathbf{q}_D)$  at temperature  $\Lambda$ , and  $f(x) = (e^x + 1)^{-1}$ . To obtain physical spin/density correlation functions, we transform the four-point susceptibility as follows [S6]:

$$\chi^{ij}(\mathbf{q}) = \sum_{\sigma_1 \sigma_2 \sigma_3 \sigma_4} \sigma_i^{\sigma_1 \sigma_3} \sigma_j^{\sigma_4 \sigma_2} \chi_{\sigma_1 \sigma_2 \sigma_3 \sigma_4}^D(\mathbf{q}). \quad (\text{S15})$$

Here,  $\sigma_i^{\sigma_1, \sigma_2}$  denote the Pauli matrices for  $i \in \{x, y, z\}$  and the identity matrix for  $i = 0$ .

#### SIII. B. Averages in momentum & spin space

The leading ordering vectors in Fig. 2 (a) of the main text were obtained with an averaging procedure on the four-point particle-hole susceptibility. For  $\mathbf{q} \in \text{BZ}$ , we

define the momentum weight function  $w(\mathbf{q})$  as

$$w(\mathbf{q}) = \left( \|\chi^D(\mathbf{q})_{\sigma_1, \dots, \sigma_4}\|_{\sigma_1, \dots, \sigma_4; 1} \right)^3, \quad (\text{S16})$$

where the norm is an absolute value norm taken over all combinations of spin indices. A meaningful expression for  $\bar{\mathbf{q}}$  can only be defined for the irreducible wedge (IBZ) defined by the triangle connecting the points  $\Gamma$ - $K$ - $M$ . We calculate the average ordering vector as

$$\bar{\mathbf{q}} = \frac{\sum_{\mathbf{q} \in \text{IBZ}} \mathbf{q} w(\mathbf{q})}{\sum_{\mathbf{q} \in \text{IBZ}} w(\mathbf{q})}. \quad (\text{S17})$$

In a similar manner, we can perform an averaging to get the relative weight in  $xx$ ,  $xy$  and  $zz$  direction (cf. Fig. 2 (b)). We first define the weight function as

$$w(i, j) = \left( \|\chi^{ij}(\mathbf{q})\|_{\mathbf{q}, 3} \right)^2, \quad (\text{S18})$$

where now the 3-norm is taken over the full BZ. Thereafter, plotting coordinates are assigned to the three com-

binations of  $i, j$  and an average similar to Eq. (S17) is performed to map each point to a specific color.

### SIII. C. Competition of density and spin ordering

As stated in the main text, we observe that at any point in the phase diagram, spin-spin correlations dominate over density-density correlations of the respective orders. We aim to visualize this behavior in Fig. S3, where we plot the weights  $w(i, j)$  of the four non-trivial spin/density correlation functions for all DW states. The weights are normalized for each value of  $\varphi$  and  $\nu$  to their maximum value. For almost all values of  $\nu$  and  $\varphi$ , the  $xx/yy$  correlations dominate. Only at  $\varphi \gtrsim 0$  and  $\varphi \approx \pi/3$ , there are small regions of dominant  $zz$  ordering.

### SIV. ANALYSIS OF SUPERCONDUCTING PHASES

In the case of the flow indicating a particle-particle instability, we employ a twofold method of analyzing the ordering tendencies. First, in the spirit of Eqs. (S13) and (S14), we calculate the particle-particle susceptibility at scale  $\Lambda_c$ :

$$\chi_{\sigma_1 \sigma_2 \sigma_3 \sigma_4}^{P, n}(\mathbf{q}_P) = \sum_{\mathbf{k}_P, \mathbf{k}'_P, \sigma_1', \sigma_2', \sigma_3', \sigma_4'} f^n(\mathbf{k}_P) L_{\sigma_1 \sigma_2 \sigma_1' \sigma_2'}^{f, P, \Lambda_c}(\mathbf{q}_P, \mathbf{k}_P) \Gamma_{\sigma_1' \sigma_2' \sigma_3' \sigma_4'}^{P, \Lambda_c}(\mathbf{q}_P, \mathbf{k}_P, \mathbf{k}'_P) L_{\sigma_3' \sigma_4' \sigma_3 \sigma_4}^{f, P, \Lambda_c}(\mathbf{q}_P, \mathbf{k}'_P) f^n(\mathbf{k}'_P), \quad (\text{S19})$$

where  $f^n(\mathbf{k})$  is a formfactor and  $L_{\sigma_1 \sigma_2 \sigma_3 \sigma_4}^{f, P, \Lambda}(\mathbf{q}^P, \mathbf{k}_1)$  refers to the particle-particle Fermi loop:

$$L_{\sigma_1 \sigma_2 \sigma_3 \sigma_4}^{f, P, \Lambda}(\mathbf{q}^P, \mathbf{k}_1) = \sum_{b_1 b_2} \frac{u_{\sigma_1 b_1}(\mathbf{k}_1) u_{\sigma_3 b_1}^*(\mathbf{k}_1) u_{\sigma_2 b_2}(\mathbf{k}_2^P) u_{\sigma_4 b_2}^*(\mathbf{k}_2^P) [f(-\epsilon_{b_1}(\mathbf{k}_1)/\Lambda) - f(\epsilon_{b_2}(\mathbf{k}_2^P)/\Lambda)]}{\epsilon_{b_1}(\mathbf{k}_1) + \epsilon_{b_2}(\mathbf{k}_2^P)}. \quad (\text{S20})$$

Second, we solve a linearized gap equation for  $\Gamma^{(4), \Lambda}$ :

$$\lambda \Delta_{\sigma_1 \sigma_2}(\mathbf{k}) = \sum_{\mathbf{k}' \sigma_3 \sigma_4 \sigma_1' \sigma_2'} \Gamma_{\sigma_1 \sigma_2 \sigma_3 \sigma_4}^{P, \Lambda}(\mathbf{q}_P = 0, \mathbf{k}, \mathbf{k}') L_{\sigma_3 \sigma_4 \sigma_1' \sigma_2'}^{f, P, \Lambda}(\mathbf{q}^P = 0, \mathbf{k}') \Delta_{\sigma_1' \sigma_2'}(\mathbf{k}'). \quad (\text{S21})$$

For numerical treatment, it is notable that the eigenproblem Eq. (S21) is non-Hermitian; and therefore not stable. So we instead perform a singular value decomposition of the matrix composed of  $\Gamma^{P, \Lambda}$  and  $L^{f, P, \Lambda}$ :

$$\hat{\Gamma}^{P, \Lambda} \hat{L}^{f, P, \Lambda} = \hat{U} \hat{\Sigma} \hat{V}^\dagger, \quad (\text{S22})$$

with singular values  $\hat{\Sigma}$  and right (left) singular vectors  $\hat{V}$  ( $\hat{U}$ ). All Fermi surface projection is encoded in the right singular vectors  $\hat{V}$ , whereas  $\hat{U}$  display the symmetry of the superconducting order parameter in the full BZ.

For further analysis of the gap symmetry, we trans-

form the singular vectors corresponding to the maximal singular values (i.e. leading singular vectors) to singlet and triplet space [S7, S8]:

$$\hat{\Delta}(\mathbf{k}) = i [\psi(\mathbf{k}) + \hat{\sigma} \cdot \mathbf{d}(\mathbf{k})] \hat{\sigma}_y, \quad (\text{S23})$$

where  $\hat{\sigma}$  is the vector of Pauli matrices.

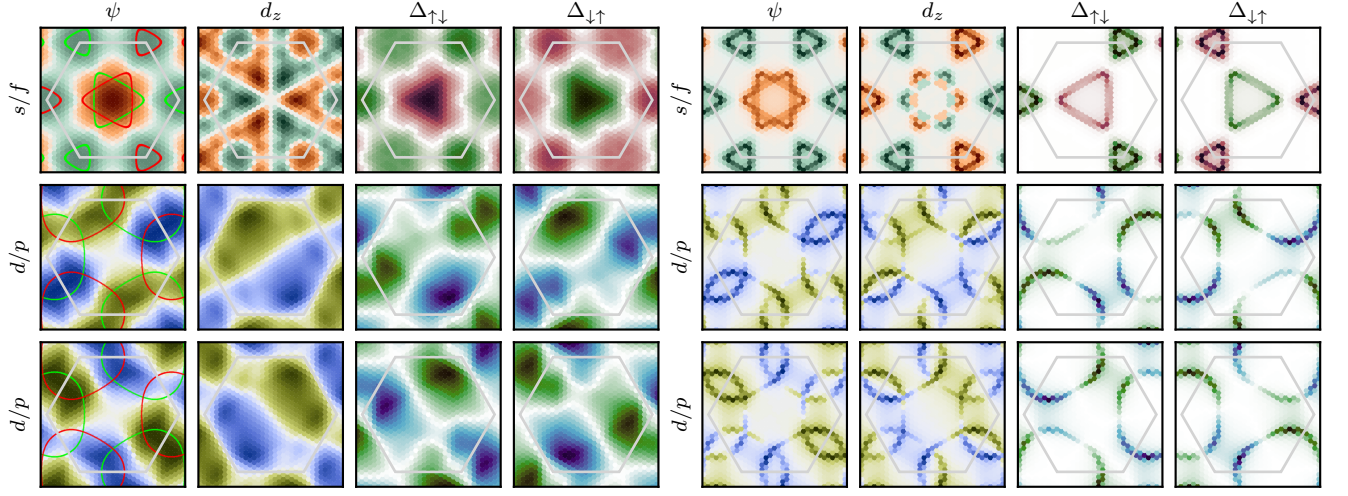

FIG. S4. **Left:** Superconducting gap functions in singlet/triplet (left two columns) and spin up/spin down (right two columns) space. The first row corresponds to an  $s/f$ -wave instability, the second and third rows to two degenerate  $d/p$ -wave instabilities. **Right:** Fermi-surface (FS) projected superconducting gap functions. Each panel is showing the same instability as on the left, with the only difference being the use of right singular vectors  $\hat{V}$  instead of left singular vectors  $\hat{U}$  in the singular value decomposition of Eq. (S22) which leads to the FS projection.

#### SIV. A. Spin-resolved gap functions

For the two points in the phase diagram where we display singlet/triplet resolved gap functions (cf. Fig. 3 of

the main text), we provide plots of the same gap functions in the spin- $z$  basis in Fig. S4. We further add the gap functions in singlet/triplet basis to the same figure to emphasize the differences.

- 
- [S1] L. Klebl, Q. Xu, A. Fischer, L. Xian, M. Claassen, A. Rubio, and D. M. Kennes, Moiré engineering of spin-orbit coupling in twisted platinum diselenide, *Electronic Structure* **4**, 014004 (2022).
  - [S2] W. Metzner, M. Salmhofer, C. Honerkamp, V. Meden, and K. Schönhammer, Functional renormalization group approach to correlated fermion systems, *Reviews of Modern Physics* **84**, 299 (2012).
  - [S3] C. Platt, W. Hanke, and R. Thomale, Functional renormalization group for multi-orbital fermi surface instabilities, *Advances in Physics* **62**, 453 (2013), <https://doi.org/10.1080/00018732.2013.862020>.
  - [S4] M. Salmhofer and C. Honerkamp, Fermionic Renormalization Group Flows: Technique and Theory, *Progress of Theoretical Physics* **105**, 1 (2001), <https://academic.oup.com/ptp/article-pdf/105/1/1/5164880/105-1-1.pdf>.
  - [S5] J. Beyer, J. B. Hauck, and L. Klebl, Reference results for the momentum space functional renormalization group (2022).
  - [S6] D. D. Scherer and B. M. Andersen, Spin-orbit coupling and magnetic anisotropy in iron-based superconductors, *Phys. Rev. Lett.* **121**, 037205 (2018).
  - [S7] M. Sigrist and K. Ueda, Phenomenological theory of unconventional superconductivity, *Rev. Mod. Phys.* **63**, 239 (1991).
  - [S8] M. Smidman, M. B. Salamon, H. Q. Yuan, and D. F. Agterberg, Superconductivity and spin-orbit coupling in non-centrosymmetric materials: a review, *Reports on Progress in Physics* **80**, 036501 (2017).
